# Supplementary material for: Resolving the Flavor Structure in the MFV-SMEFT
Source: arXiv:2212.02532 source file (2022-12-05)
Supplement: Supplementary file 1 [file appendix.tex]

\section{XXX}\label{app:xxx}
